# Supplementary material for: Impact of Redundancy on Resilience in Distributed Optimization and Learning
Source: arXiv:2211.08622 source file (2023-12-14)
Supplement: Supplementary file 1 [file supplement-exp.tex]

\section{Numerical examples}
\label{appdx:exp-numerical}

We present a group of simulation results applying our algorithm framework to the problems of (deterministic) \textit{distributed linear regression}. Specifically, we study the behavior of Algorithm~\ref{alg} according to our theoretical results in Section~\ref{sec:full-grad}, including the special cases.

\subsection{Problem Description}

Consider a synchronous server-based system, where $n=10$ and $d=2$. Each agent $i\in\{1,...,n\}$ has a data point represented by a triplet $(A_i,B_i,N_i)$ where $A_i$ is a $d$-dimensional row vector, $B_i\in\R$ is a response, and $N_i\in\R$ is a noise value. Specifically, for all $i\in\{1,...,n\}$, 
\begin{equation}
    B_i=A_ix^*+N_i ~ \text{ where } ~x^*=\begin{pmatrix}1\\1\end{pmatrix}.
\end{equation}
The collective data is represented by a triplet of matrices $(A, \, B, \, N)$ where the $i$-th row of $A$, $B$, and $N$ are equal to $A_i$, $B_i$ and $N_i$, respectively. The specific values are as follows.
\begin{equation}
    A=\begin{pmatrix}
        1 & 0 \\
        0.8 & 0.5 \\
        0.5 & 0.8 \\
        0 & 1 \\
        -0.5 & 0.8 \\
        -0.8 & 0.5 \\
        0.3 & -0.7 \\
        0.7 & 0.3 \\
        0.3 & 0.7 \\
        0.7 & -0.3
    \end{pmatrix}, ~ 
    B=\begin{pmatrix}
        %0.91078179 \\  1.33487616 \\ 1.33758823 \\ 1.00334385 \\ 0.21424485 \\ -0.36153888
        0.9108 \\  1.3349 \\ 1.3376 \\ 1.0033 \\ 0.2142 \\ -0.3615 \\ -0.3974 \\ 0.9967 \\ 1.0052 \\ 0.3947
    \end{pmatrix}, ~ \text{ and }
    N=\begin{pmatrix}
        %-0.08921821 \\0.03487616\\0.03758823\\0.00334385\\-0.08575515\\-0.06153888
        -0.0892 \\0.0349 \\0.0376\\0.0033\\-0.0858\\-0.0615\\0.0026\\-0.0033\\0.0052\\-0.0053
    \end{pmatrix}.
\end{equation}
It should be noted that
\begin{align}
    B = A x^{*} + N. \label{eqn:set_equations}
\end{align}
We let $A_S$, $B_S$ and $N_S$ represent matrices of dimensions $\mnorm{S} \times 2$, $\mnorm{S} \times 1$ and $\mnorm{S} \times 1$ obtained by stacking the rows $\{A_i, \, i \in S \}$, $\{B_i, \, i \in S \}$ and $\{N_i, \, i \in S\}$, respectively, in the increasing order of $i$. From~\eqref{eqn:set_equations}, observe that for every non-empty set $S$,
\begin{align}
    B_S = A_S x^{*} + N_S. \label{eqn:set_equations-2}
\end{align}
Recall from basic linear algebra that if $A_S$ is full-column rank, i.e., $\rank{A_S} = d = 2$ then $x^*$ is the unique solution of the set of equations in~\eqref{eqn:set_equations-2}. 
% Note that for every set $S$ with $\mnorm{S} \geq n-2f = 6 - 2 = 4$, the matrix $A_S$ is full rank. Specifically,
Note that in this example, for every set $S$ with $\mnorm{S} \geq 2$, the matrix $A_S$ is full rank. Specifically,
\begin{align}
    \rank{A_S} = d = 2, \quad \forall S \subseteq \{1, \ldots, \, 10\}, ~ \mnorm{S} \geq 2. \label{eqn:exp_full_rank}
\end{align}

In this particular distributed optimization problem, each agent $i$ has a quadratic cost function defined to be 
\[Q_i(x)=(B_i-A_ix)^2, \quad \forall x \in \R^2.\] 
For an arbitrary non-empty set of agents $S$, we define 
\begin{align}
Q_S(x) = \sum_{i\in S}Q_i(x) = \sum_{i \in S}\left(B_i-A_ix \right)^2 = \norm{B_S-A_Sx}^2, \quad \forall x \in \R^2. \label{def:exp_Q_S}
\end{align}
As matrix $A_S$ is full rank for every $S$ with $\mnorm{S} \geq 2$,

\comment{This result below is wrong. (cf. PODC appendix)}
\begin{align}
    \arg \min_{x \in \R^2} Q_S(x) = \arg \min_{x \in \R^2} \norm{B_S-A_Sx}^2 = \left(x ~ \vline ~ A_S x = B_S \right). \label{eqn:solve_Q_S}
\end{align}
Therefore, $Q_S(x)$ has a unique minimum point when $\mnorm{S} \geq 2$. Henceforth, we write notation $\arg \min_{x \in \R^2}$ simply as $\arg \min$, unless otherwise stated.

\subsection{Redundancy property and parameters}

\begin{figure}[t]
    \centering
    \includegraphics[width=.4\textwidth]{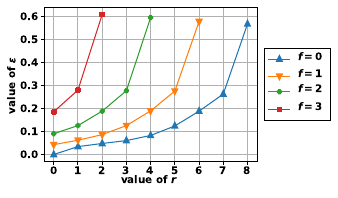}
    \caption{Trade-off between $\epsilon$, $f$ and $r$ for the numerical example. The total number of agents $n=10$. The figure is the same as in Figure~\ref{fig:trade-off-main}.}
    \label{fig:trade-off}
\end{figure}

In the following experiments, we choose $f=0,1,2$ and $r=0,1,2$, with various combinations. In each execution, we always designate the first $f$ agents to be Byzantine faulty. It can be verified first that the agents' cost functions satisfy $(f,r;\epsilon)$-redundancy property. The value of $\epsilon$ can be computed by the following steps, similar to the steps in the previous section:
\begin{enumerate}
    \item For each set $S\subset\{1,...,n\}$ with $\mnorm{S}=n-f$, compute $x_S\in\R^2$ such that $B_S=A_Sx_S$. Note that due to \eqref{eqn:solve_Q_S}, $x_S=\arg\min Q_S(x)$.
    \item For each set $S\subset\{1,...,n\}$ with $\mnorm{S}=n-f$, do the following:
    \begin{enumerate}
        \item For each set $\widehat{S}\subseteq{S}$ with $\mnorm{\widehat{S}}\geq n-r-2f$, compute $x_{\widehat{S}}$ such that $B_{\widehat{S}}=A_{\widehat{S}}x_{\widehat{S}}$. By \eqref{eqn:solve_Q_S}, $x_{\widehat{S}}=\arg\min Q_{\widehat{S}}(x)$.
        \item Compute $\epsilon_S=\max_{\widehat{S}\subseteq S,\mnorm{\widehat{S}}\geq n-2f-r}\norm{x_S-x_{\widehat{S}}}$.
    \end{enumerate}
    \item Finally, compute $\epsilon=\max_{S,\mnorm{S}=n-f}\epsilon_S$.
\end{enumerate}
The values of $\epsilon$ with different $f$ and $r$ are presented in Figure~\ref{fig:trade-off}. We can see that the larger the values of $f$ and $r$, the larger the value of $\epsilon$, indicating the less accurate an algorithm can we expect. 

We simulate the distributed gradient-descent-based algorithm according to Theorem~\ref{thm:async-fault-toler} in Section~\ref{sec:full-grad}. The algorithm ignores the input from $r$ slowest agents in each iteration, and uses the CGE GAR to tolerate Byzantine agents. Let $\H=[n]\backslash[f]$ be the set of non-faulty agents. From \eqref{eqn:solve_Q_S} we can compute the minimum point of the aggregate cost function of non-faulty agents $x_\H=x_S=\sum_{i\in\H}Q_i(x)$.

For each agent $i$, its cost function $Q_i(x)$ has Lipschitz continuous gradients, i.e., satisfies Assumption~\ref{assum:lipschitz}, with Lipschitz coefficient $\mu=2\overline{v}_i$, where $\overline{v}_i$ denotes the largest eigenvalue of $A_i^TA_i$. Also, for the set $S$, their average cost function $(1/\mnorm{S})Q_S(x)$ is strongly convex, i.e., satisfies Assumption~\ref{assum:strongly-convex-ft}, with strong convexity coefficient $\gamma=2\underline{v}_S/\mnorm{S}$, where $\underline{v}_S$ is the smallest eigenvalue of $A_S^TA_S$. The derivations of computing these two coefficients can be found in \cite[Section 10]{gupta2019byzantine}. We can compute the values of the coefficients accordingly: $\mu=2$; $\gamma =0.788, 0.588, 0.439$ when $f=0,1,2$, respectively.

We use the following parameters to implement the algorithm. In update rule \eqref{eqn:update}, we use step size $\eta_t=1.5/(t+1)$ for iteration $t=0,1,...$, which satisfies the conditions $\sum_{t=0}^\infty\eta_t=\infty$ and $\sum_{t=0}^\infty\eta_t^2=3\pi^2/8<\infty$  (see~\cite{rudin1964principles}). We assume the convex compact $\W\subset\R^d$ to be a 2-dimensional hypercube $[-1000,1000]^2$. Note that $x_\H\in\W$. In all simulations presented, the initial estimate $x^0=(0,0)^T$. In every execution, we observe that the iterative estimates produced by the algorithm practically converge after 400 iterations. Thus, to measure the approximate result outputted by the algorithm, we use $x_\textrm{out}=x^{500}$. 

Two types of fault behaviors are simulated: (i) \textit{gradient-reverse}: the faulty agent \textit{reverses} its true gradient. Suppose the correct gradient of a faulty agent $i$ at iteration $t$ is $s_i^t$, the agent $i$ will send the incorrect gradient $g_i^t=-s_i^t$ to the server.
(ii) \textit{random}: the faulty agent sends a randomly chosen vector in $\mathbb{R}^d$. In our experiments, the faulty agent in each iteration chooses i.i.d. Gaussian random vector with a mean of 0 and an isotropic covariance matrix with a standard deviation of 200.

\subsection{Experiment results and discussions}

The outputs with different values of $f$ and $r$ are presented in Table~\ref{tab:results} alongside with plain gradient descent output ($f=r=0$) for comparison. Note that $\dist{x_\H}{x_\textrm{out}}=\norm{x_\H-x_\textrm{out}}$. In all executions, $\dist{x_\H}{x_\textrm{out}}<\D^*$ as indicated by Theorem~\ref{thm:async-fault-toler}. The values of $\D^*$ are presented below:
\begin{center}
    \begin{tabular}{c|ccc}
         & $r=0$ & $r=1$ & $r=2$ \\
        \hline
        $f=0$ & 0 & 0.207 & 0.385 \\
        $f=1$ & 0.369 & 0.670 & 0.957 \\
        $f=2$ & 1.251 & 1.748 & 2.467 \\
    \end{tabular}
\end{center}

We also plot the processes of Algorithm~\ref{alg} solving the numerical examples of some of these experiments, namely the cases when $f=1$ and $2$, in Figure~\ref{fig:a}, with details of the first 150 iterations of each execution. The process when $f=r=0$, i.e., the synchronous fault-free case is also presented for comparison purposes. These plots show that in order to be resilient against Byzantine agents and stragglers, the convergence speed is slightly slowed down and there exists a gap between the algorithm's output and the true solution, echoing the error bound we obtained in Section~\ref{sec:full-grad}.

\begin{table*}[t]
    \centering
    \caption{Outputs of Algorithm~\ref{alg} when solving the distributed linear regression in Appendix~\ref{appdx:exp-numerical}. GAR in use: summing $n-r$ gradients when $f=0$, and CGE gradient filter when $f=1,2$. %The resilience of the algorithm is shown by the distance between the outputs and the actual solution to the problem. The true solution to optimization problems $x_\H$ are also listed. %Recall that $x_{\mathrm{out}} = x^{500}$ and $\dist{x_\H}{x_{\mathrm{out}}}=\norm{x_\H-x_{\mathrm{out}}}$.
    }
    \footnotesize
    \begin{tabular}[t]{c|c|ccc|c}
        & & $r=0$ & $r=1$ & $r=2$ & $x_\H$ \\
        \hline
        \multirow{2}{*}{$f=0$}& $x_\textrm{out}$ & $\begin{pmatrix}1.0117 \\ 0.9883\end{pmatrix}$ & $\begin{pmatrix}1.0152 \\ 0.9891\end{pmatrix}$ & $\begin{pmatrix}1.0311\\ 0.9872\end{pmatrix}$ & \multirow{2}{*}{$\begin{pmatrix}1.0117 \\ 0.9883\end{pmatrix}$} \\
        & $\dist{x_\H}{x_\textrm{out}}$ & $\sim0$ & $3.66\times10^{-3}$ & $1.95\times10^{-2}$ \\
        \hline
        $f=1$ & $x_\textrm{out}$ & $\begin{pmatrix}1.0460\\ 0.9883\end{pmatrix}$ & $\begin{pmatrix}1.0363\\ 0.9994\end{pmatrix}$ & $\begin{pmatrix}1.0346\\ 0.9934\end{pmatrix}$ & \multirow{4}{*}{$\begin{pmatrix}1.0460\\ 0.9883\end{pmatrix}$} \\
        \textit{grad-rev} & $\dist{x_\H}{x_\textrm{out}}$ & $1.48\times10^{-5}$ & $1.47\times10^{-2}$ & $1.24\times10^{-2}$ \\
        \cline{1-5}
        $f=1$ & $x_\textrm{out}$ & $\begin{pmatrix}1.0459\\ 0.9883\end{pmatrix}$ & $\begin{pmatrix}1.0466\\ 0.9846\end{pmatrix}$ & $\begin{pmatrix}1.0403\\ 0.9923\end{pmatrix}$ \\
        \textit{random} & $\dist{x_\H}{x_\textrm{out}}$ & $5.42\times10^{-5}$ & $3.71\times10^{-3}$ & $6.93\times10^{-3}$ \\
        \hline
        $f=2$ & $x_\textrm{out}$ & $\begin{pmatrix}1.0067\\ 0.9621\end{pmatrix}$ & $\begin{pmatrix}1.0138\\ 0.9789\end{pmatrix}$ & $\begin{pmatrix}0.9891\\ 1.0090\end{pmatrix}$ & \multirow{4}{*}{$\begin{pmatrix}1.0445\\ 0.9876\end{pmatrix}$} \\
        \textit{grad-rev} & $\dist{x_\H}{x_\textrm{out}}$ & $4.56\times10^{-2}$ & $3.19\times10^{-2}$ & $5.94\times10^{-2}$ \\
        \cline{1-5}
        $f=2$ & $x_\textrm{out}$ & $\begin{pmatrix}1.0444\\ 0.9876\end{pmatrix}$ & $\begin{pmatrix}1.0376\\ 0.9961\end{pmatrix}$ & $\begin{pmatrix}1.0296\\ 1.0030\end{pmatrix}$ \\
        \textit{random} & $\dist{x_\H}{x_\textrm{out}}$ & $6.00\times10^{-5}$ & $1.10\times10^{-2}$ & $2.14\times10^{-2}$ \\
    \end{tabular}
    \label{tab:results}
\end{table*}

\begin{figure*}[t]
    \centering
    \includegraphics[width=\textwidth]{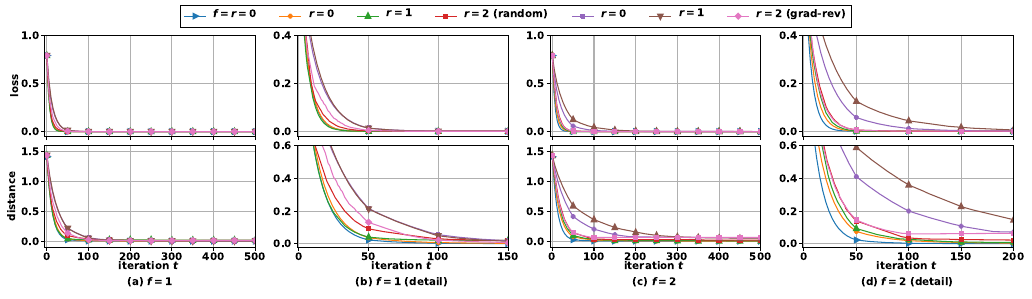}
    \caption{Changes in aggregate cost $\sum_{i\in\H}Q_i(x^t)$, and $\dist{x^t}{x_\H}$, versus the number of iterations with Algorithm~\ref{alg} solving the numerical example. %Columns (a) and (c) are {for the first 500 iterations}, while (b) and (d) are details from the initial iterations. The results for fault-free synchronous gradient descent ($f=r=0$) is also presented for comparison.
    }
    \label{fig:a}
\end{figure*}
