# Supplementary material for: Impact of Redundancy on Resilience in Distributed Optimization and Learning
Source: arXiv:2211.08622 source file (2023-12-14)
Supplement: Supplementary file 3 [file supplement-proof.tex]

\section{Proof for Theorem~\ref{thm:necc}}
\label{appdx:proof-necessity}

\begin{proof} 
To prove the theorem we present a scenario where the agents' cost functions are scalar functions, i.e., $d = 1$ and for all $i$, $Q_i: \R \to \R$, and the minimum point of an aggregate of one or more agents' cost functions is uniquely defined. We also assume that stragglers are extreme enough that none of their information can be received by the server. Obviously, if a condition is necessary in this particular scenario then it is also necessary in the general case we consider.

% Second, our arguments can be easily extended for the case when $d > 1$. As the theorem is rendered vacuous when $f = 0$, we assume that $f > 0$.\\

To prove the necessary condition, we also assume that the server has full knowledge of all the agents' cost functions. This may not hold true in practice, where instead the server may only have partial information about the agents' cost functions. Indeed, this assumption forces the Byzantine faulty agents to a priori fix their cost functions. However, in reality the Byzantine agents may send arbitrary information over time to the server that need not be consistent with a fixed cost function. Thus, necessity of $(2f,\epsilon)$-redundancy under this strong assumption implies its necessity in general. 

The proof is by contradiction. Specifically, we show that \textit{if the cost functions of non-faulty agents do not satisfy the $(f,r;\epsilon)$-redundancy property then there cannot exist a \emph{deterministic} $(f,r;\epsilon)$-resilient distributed optimization algorithm.}
% \begin{quote}
%     %If the non-faulty cost functions satisfy $(2f,\epsilon)$-redundancy for some $\epsilon$, deterministic distributed optimization algorithm cannot guarantee $(f,\epsilon-\delta)$-resilience, for any $\delta$, $0\geq\delta<\epsilon$.
%     %For some $\epsilon>0$, if the non-faulty cost functions do not satisfy $(2f,\epsilon)$-redundancy, deterministic distributed optimization algorithm cannot guarantee $(f,\epsilon)$-resilience.
%     %, for any $\delta$, $0\geq\delta<\epsilon$.
% 
% \end{quote}
% We show that the above statement is
% 

Recall that we have assumed that for a non-empty set of agents $T$ the aggregate cost function $\sum_{i \in T} Q_i(x)$ has a unique minimum point. To be precise, for each non-empty subset of agents $T$, we define
\[\textstyle x_T = \arg \min_x \sum_{i \in T} Q_i(x).\]

Suppose that the agents' cost functions \textbf{do not} satisfy the $(f,r;\epsilon)$-redundancy property stated in Definition~\ref{def:redundancy}. 
Then, there exists a real number $\delta > 0$ and a pair of non-empty subsets of non-faulty agents $S, \, \widehat{S}$ with $\widehat{S} \subset S$, $\mnorm{S} = n-f$, and $n-2f-r \leq \mnorm{\widehat{S}} < n-f$ such that
% there exits a pair of sets $S, \, \widehat{S} \subseteq \{1, \ldots, \, n\}$ with $\mnorm{S} \geq n-f$, $\mnorm{\widehat{S}} \geq n-2f$ and $\widehat{S} \subseteq S$ such that 
% \begin{align*}
%     \norm{x_{\widehat{S}} - x_S} = \epsilon + \delta
% \end{align*}
% where $\delta > 0$. As shown in Lemma~\ref{lem:red_imply} presented in Appendix~\ref{app:red_imply}, the above implies that 
% there exists a pair of sets $T, \, \widehat{T} \subset \{1, \ldots, \, n\}$ with $\mnorm{T} = n-f$, $\mnorm{\widehat{T}} = n-2f$ and $\widehat{T} \subset T$ such that
\begin{align}
    \norm{x_{\widehat{S}} - x_S} \geq \epsilon + \delta. \label{eqn:no_red_asp}
\end{align}
% \textcolor{red}{\bf ++++ editing +++++ }
% \\
% For a subset $S_0$ comprising of $n-2f$ non-faulty agents, suppose that the minimum point of the aggregated cost function of the agents in $S_0$ is unique. We denote
% \begin{equation}
%     x_0=\arg\min\sum_{i\in S_0}Q_i(x).
% \end{equation}
% Let set $S_1$ denote the remaining $f$ non-faulty agents. Suppose that the minimum point of the aggregated cost function of all the non-faulty agents in $S_0 \cup S_1$ is also unique. We denote
% % A set $S_1\subset\{1,...,n\}\backslash S_0$ of $t$ agents has
% \begin{equation}
%     x_1=\arg\min_x\sum_{i\in S_0\cup S_1}Q_i(x)
% \end{equation}
% As we have assumed that the non-faulty agents do not satisfy the $(2f,\epsilon)$-redundancy, there exist the aforementioned sets $S_0$ and $S_1$, and $\delta > 0$, such that $x_0$ is $\epsilon + \delta$ distance away from $x_1$, i.e.,
% \begin{align*}
%     \norm{x_0 - x_1} = \epsilon + \delta.
% \end{align*}
Now, suppose that $n - f - r - \mnorm{\widehat{S}}$ agents in the remainder set $\{1, \ldots, \, n\} \setminus S$ are Byzantine faulty. Let us denote this set of faulty agents by $\B$. Note that $\B$ is non-empty with $\mnorm{\B} = n - f - r-\mnorm{\widehat{S}} \leq f$. 
% Now, let all the remaining $f$ agents in the set $\B = \{1, \ldots, \, n\} \setminus S$ be Byzantine faulty. 
Similar to the non-faulty agents, the faulty agents send to the server cost functions that are scalar, and the aggregate of one or more agents' cost functions in the set $S \cup \B$ is unique\footnote{For otherwise Byzantine agents would have been spotted by the server and become useless.}. Suppose the set of agents $T=S\backslash\widehat{S}$. We replace arbitrary $\mnorm{\B}$ agents in $T$ with $\B$, and denote the new set of agents as $T'$.

The cost functions of faulty agents can be arbitrary. We would like to choose those functions of the faulty agents such that
% \begin{quote}
the aggregate cost function of the agents in the set $\widehat{S}\cup T'$ minimizes at a unique point $x_{\widehat{S}\cup T'}$ which is $\norm{x_{\widehat{S}} - x_{S}}$ distance away from $x_{\widehat{S}}$, similar to $x_S$, but lies on the other side of $x_{\widehat{S}}$ as shown in the figure below. Note that it is always possible to pick such functions for the faulty agents. For example, suppose $S=\{1,2,3,4\}$, $\widehat{S}=\{1,2\}$, $f=r=1$. $Q_1(x)=Q_2(x)=Q_3(x)=x^2$, and $Q_4(x)=(x-1)^2$. $\B$ should contain 1 agent, denote it as agent 5. If $T'=\{3,5\}$, we can choose $Q_5(x)=(x+1)^2$. If $T'=\{4,5\}$, we can choose $Q_5(x)=x^2+4x$. Either way, $x_{\widehat{S}}=0$, $x_S=1/4$, and $x_{\widehat{S}\cup T'}=-1/4$.
% \end{quote}

% The remaining $f$ agents denoted by set $S_2 = \{1,...,n\} \setminus S_0 \setminus S_1$ are Byzantine faulty. A Byzantine faulty agent $i \in S_2$ chooses a cost function $Q_i(x): \R \to \R$ with similar properties as a non-faulty cost function such that the following conditions hold true. 
% \begin{itemize}
%     \item The minimum point of the aggregated cost function of the agents in $S_0 \cup S_2$ is unique. We denote 
%     \begin{equation*}
%         x_2=\arg\min_x\sum_{i\in S_0\cup S_2}Q_i(x).
%     \end{equation*}
%     \item The distance between $x_0$ and $x_2$ is $\epsilon + \delta$, i.e., $\norm{x_0 - x_2} = \epsilon + \delta$. However, the point $x_2$ lies in the other half of the real line $\R$ than the point $x_1$ as shown in the figure below.
% \end{itemize}

\begin{center}
    \includegraphics[width=.4\textwidth]{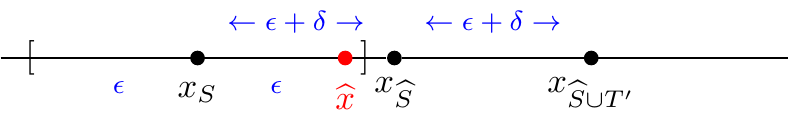}
\end{center}

\noindent Note that the distance between the two points $x_S$ and $x_{\widehat{S}\cup T'}$ is $2\epsilon + 2\delta$, i.e.,
\begin{align}
    \norm{x_S - x_{\widehat{S}\cup T'}} = 2\epsilon + 2\delta. \label{eqn:dist_x1_x2}
\end{align}
% The functions can be constructed. Suppose each cost function $Q_i(x)$, $i\in S_0$ satisfies $Q_i(x)=Q_i(2x_0-x)$. To satisfy the conditions stated above, for every cost function $Q_i(x)$, $i\in S_1$, one can construct another function $Q_j(x)=Q_i(2x_0-x)$, to be the cost function of an agent $j\in S_2$. \\%(See Figure~\ref{fig:constructQ})\\
%$\distance(x_0,x_1)=\distance(x_0,x_2)=\epsilon$. And functions in $S_0$, $S_1$, and $S_2$ are symmetric with respect to $x_0$, meaning for any $Q_i$ in $X_0$, $Q_i(x)=Q_i(2x_0-x)$, and for any $Q_i\in S_1$ and $Q_j\in S_2$, $Q_i(x)=Q_j(2x_0-x),~\forall x$. \\
% We now show below, by contradiction, that there cannot exist a deterministic $(f, \, \epsilon)$-resilient algorithm.\\

Now, suppose, toward a contradiction, that there exists an $(f, r; \epsilon)$-resilient deterministic optimization algorithm named $\Pi$. As the identity of Byzantine faulty agents is a priori unknown to the server, and the cost functions sent by the Byzantine faulty agents have similar properties as the non-faulty agents, 
% and the faulty cost functions are assumed differentiable and convex, 
the server cannot distinguish between the following two possible scenarios; i) $S$ is the set of non-faulty agents, and ii) $\widehat{S}\cup T'$ is the set of non-faulty agents. Note that both the sets $S$ and $\widehat{S}\cup T'$ contain $n-f$ agents. 
% Thus, the output of algorithm $\Pi$ assumed to be $(f, \, \epsilon)$-resilient should be located within $\epsilon$ distance from the minimum point of the aggregate cost functions of the non-faulty agents in both the scenarios. \\

As the cost functions received by the server are identical in both of the above scenarios, being a deterministic algorithm, $\Pi$ should have identical output in both the cases. We let $\widehat{x}$ denote the output of $\Pi$. In scenario (i) when the set of honest agents is given by $S$ with $\mnorm{S} = n-f$, as $\Pi$ is assumed $(f,r;\epsilon)$-resilient, by Definition~\ref{def:resilience} the output
\begin{align}
    \widehat{x} \in  [x_S - \epsilon, \, x_S + \epsilon] \label{eqn:scn_1}
\end{align}
as shown in the figure above. Similarly, in scenario (ii) when the set of honest agents is $\widehat{S}\cup T'$ with $\mnorm{\widehat{S}\cup T'} = n-f$,
\begin{align}
    \widehat{x} \in  [x_{\widehat{S}\cup T'} - \epsilon, \, x_{\widehat{S}\cup T'} + \epsilon]. \label{eqn:scn_2}
\end{align}
However,~\eqref{eqn:dist_x1_x2} implies that~\eqref{eqn:scn_1} and~\eqref{eqn:scn_2} cannot be satisfied simultaneously. That is, if $\Pi$ is $(f,r;\epsilon)$-resilient in scenario (i) then it cannot be so in scenario (ii), and vice-versa. This contradicts the assumption that $\Pi$ is $(f,r;\epsilon)$-resilient.

Note that the above argument stands no matter which group of agents are stragglers (less than $r$), since the existence of stragglers does not change the supposedly \textit{correct} minimum $x_S$ or $x_{\widehat{S}\cup T'}$, the minimum of aggregate of non-faulty cost functions. \qedhere
\end{proof}
